# Supplementary material for: Hallucination In Object Detection -- A Study In Visual Part Verification
Source: arXiv:2106.02523 source file (2021-06-04)
Supplement: Supplementary file 1 [file appendix.tex]

\section{Appendix}

\subsection{Evaluating context with BikeParts}
Similar to hiding BG and FG experiment on COCO dataset, BikeParts dataset is also used to evaluate the context usage of detectors. For this experiment, we choose Faster RCNN and RetinaNet since they have similar performance in terms of AP, meanwhile, different in terms of $F_{vv}$ and context usage. Note that, the experiments are evaluated on test set with intact and damaged labels. To keep the effect of localization minimal, we set the IoU threshold as 0.25.

\textbf{Hiding BG.}
Both two-stage and single-stage networks are affected by context changes (in~\fig{3in1} (left)). Faster RCNN without any context achieves 50\% of accuracy and reaches approximately 98\% of accuracy with the full context. Likewise, context adds the accuracy of RetinaNet by 34.5\%. Faster RCNN and RetinaNet leverage their performances by using contextual information. Interestingly, RetinaNet, full-context detectors, attains higher results than Faster RCNN when there is no context around the object. BikeParts dataset has not only contextual bias but also location bias and they together play a role on the performance.

% Paragraph goal: Class specific results\\
% Keywords: class 1,2,3,4,5\\
% Conclusion: ….\\

\textbf{Hiding FG.} 
In~\fig{3in1} (right), RetinaNet outperforms Faster RCNN by roughly 10\% when there is only contextual information available. RetinaNet recovers the performance quicker than Faster RCNN when showing more object fragments to the network and revealing 10 pixels from each side already makes RetinaNet to reach 90\% of accuracy. Displaying 50 pixels from each side results in perfect solution for both methods. 
BikeParts dataset consists of many small bike parts such as bell, back light and reflector. Hence, detectors starts with low accuracy when the object is hidden completely. 
To parallel to COCO experiments, the BikeParts dataset also show that deep object detectors are sensitive to context.

% Paragraph goal: Class specific results\\
% Keywords: class 1,2,3,4,5\\
% Conclusion: ….\\

\subsection{Evaluating the effect of location}
% \textcolor{red}{****will be added, double checking the results****}\\
% Paragraph goal: Setup\\
% Keywords: BGhiding, hyperparams, only testing, moving object location\\
% Conclusion: we do like this.\\
In BikeParts dataset, it is clearly seen that dataset not only have contextual bias but also location bias, see~\fig{avg_bike}. In this experiment, we increase the context size incrementally as it is done in hiding BG experiment but only with a difference: we also shift the location of the object to the opposite direction from x and y-axis. Namely, information about parts is kept but shifted to the different location. The performance is evaluated for the context size $\in \{0,5,10,25,50,100,150,200,250,300,350 \}$.

In~\fig{3in1} (middle), the performances of RetinaNet and Faster RCNN drastically drop from 64\% to 13\% and 50\% to 12\% respectively. As it is shown in \cite{kayhan2020translation, islam2020much}, CNNs can exploit the location and learn location specific filters. In this experiment, it can be argued that deep detectors learn the location bias in addition to contextual bias. Even if the context around the object is increased, the detector performances do not arrive the peak value fast. When the context size is more than 300 pixels, both detectors reach over 95\% of accuracy. The improvement is expected since the context around the object is big and accordingly the location shift is small. The experiment indicates that detectors use the contextual and location biases from dataset.

% \begin{figure}
% 	\centering
% 	\begin{tabular}{c@{}c}
% 	\includegraphics[width=0.95\linewidth]{images/Hide_BG_all_bike_loc_shift.pdf}
% 	\end{tabular}
% 	\caption{}
% 	\label{fig:loc_shift}
% \end{figure}

% Paragraph goal: BG Blackout with bikeparts\\
% Keywords: moving the location of the part\\
% Conclusion: they are also biased to the location\\
